# Supplementary material for: Correlation between 2D Square Ice and 3D Bulk Ice by Critical Crystallization Pressure
Source: arXiv:2602.01520 source file (2026-02-02)
Supplement: Supplementary file 1 [file Supporting_Information.pdf]

# Correlation between 2D Square Ice and 3D Bulk Ice by Critical Crystallization Pressure: Supporting Information

Zhen Zeng[1], Kai Sun[1], Rui Chen[1], Mengshan Suo[1], Zhizhao Che[*2], and Tianyou Wang[†2]

[1]State Key Laboratory of Engines, Tianjin University, Tianjin, 300350, China.
[2]State Key Laboratory of Engines & National Industry-Education Platform of Energy Storage, Tianjin University, Tianjin, 300350, China.

July 16, 2024

[*]Corresponding author, Email: chezhizhao@tju.edu.cn
[†]Corresponding author, Email: wangtianyou@tju.edu.cn

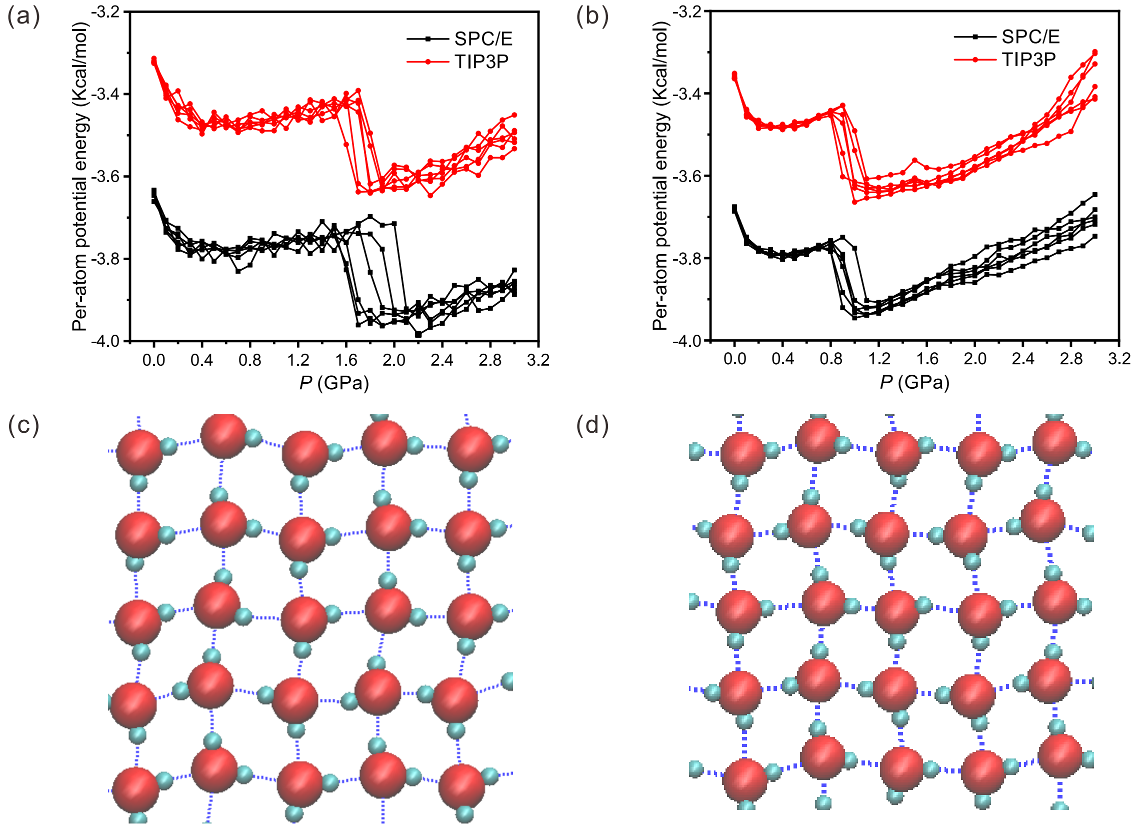


Figure S1: (a) Variation of the potential energy of the confined water during the pressurization process when the size of graphene sheets is 26.6 Å × 21.9 Å. (b) Variation of the potential energy of the confined water during the pressurization process when the size of graphene sheets is 68.0 Å × 56.0 Å. (c)–(d) Icing structures for the TIP3P water model when the sizes of graphene sheets are 26.6 Å × 21.9 Å and 68.0 Å × 56.0 Å, respectively.

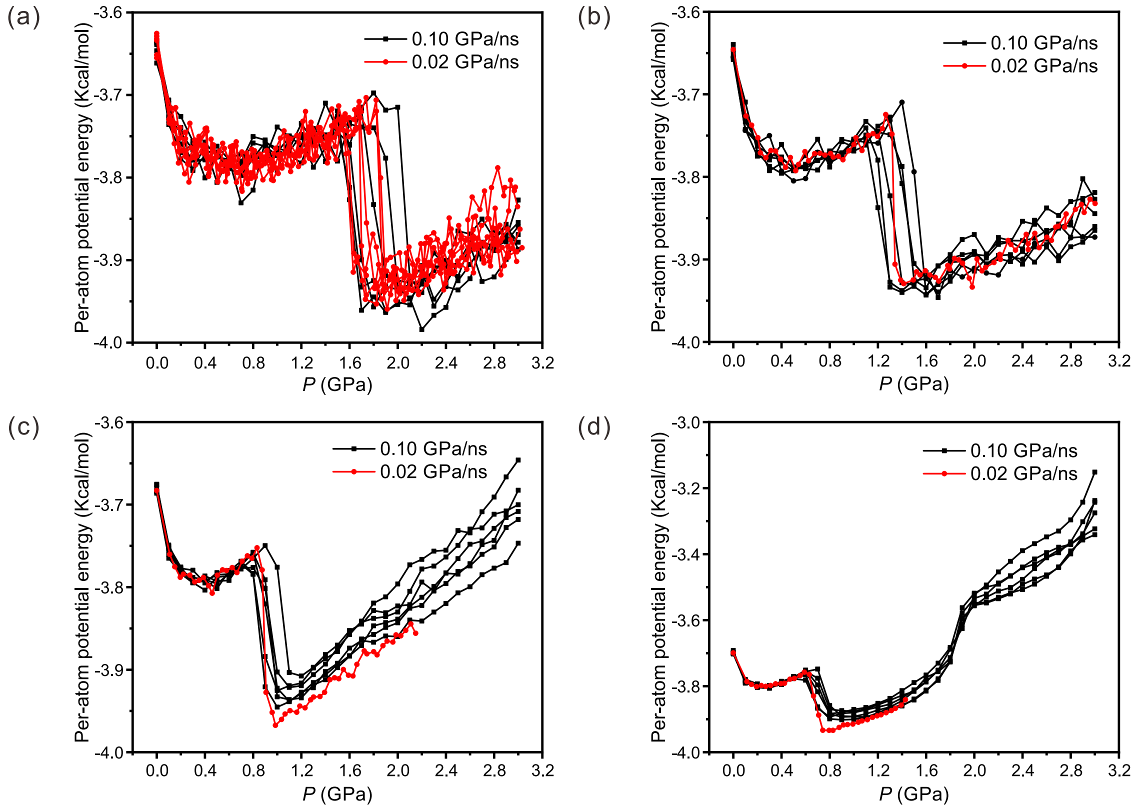


Figure S2: Variation of the potential energy of the confined water at different pressurization rates (0.02 GPa/ns and 0.10 GPa/ns) during the pressurization process (the width of the capillary $h = 9.0$ Å). (a) – (d) The size of graphene sheets is 26.6 Å × 21.9 Å, 42.5 Å × 35.0 Å, 68.0 Å × 56.0 Å, 108.8 Å × 89.6 Å, respectively.

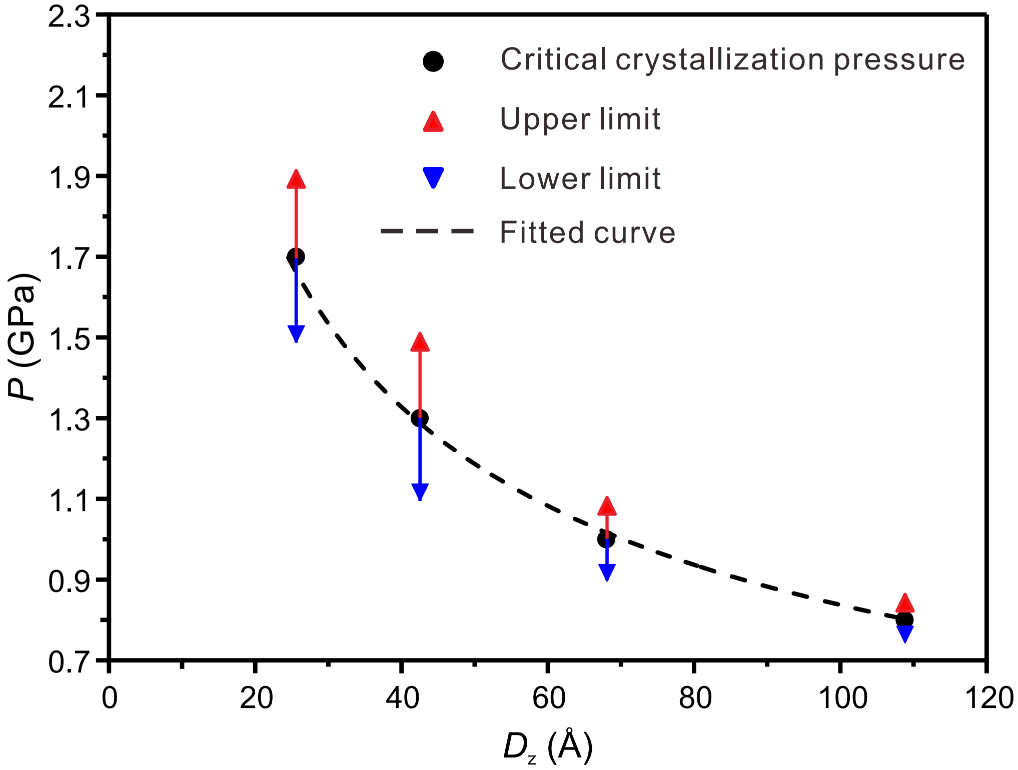


Figure S3: Critical crystallization pressure as a function of $D_z$. The red arrows represent the upper limit of critical crystallization pressure, the blue arrows represent the lower limit of critical crystallization pressure, the black dots represent the average critical crystallization pressure, and the black dashed curve is the fitted curve of the average critical crystallization pressure.

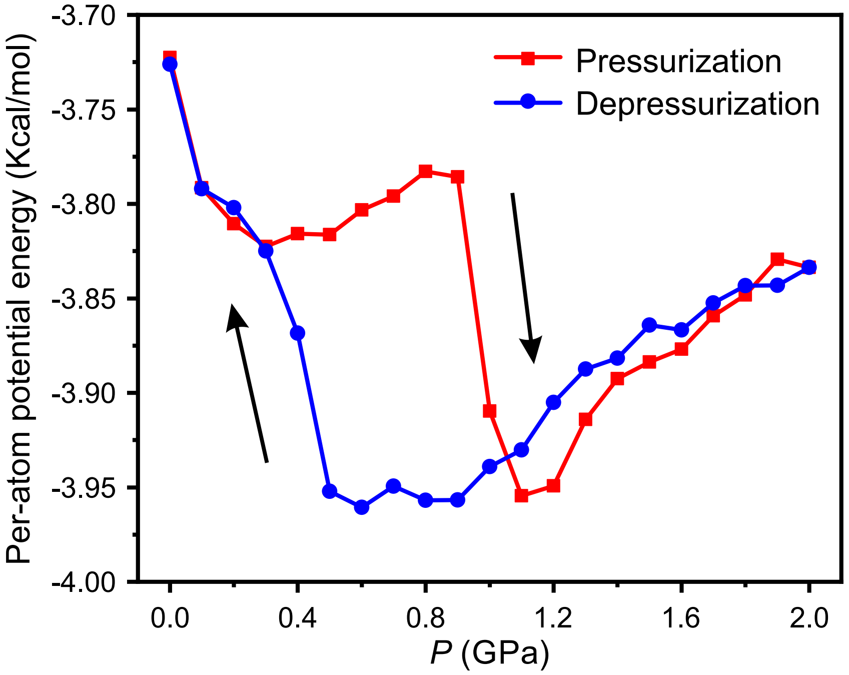


Figure S4: Pressurization/depressurization process (68.0 Å × 56.0 Å for $D_z \times D_x$).

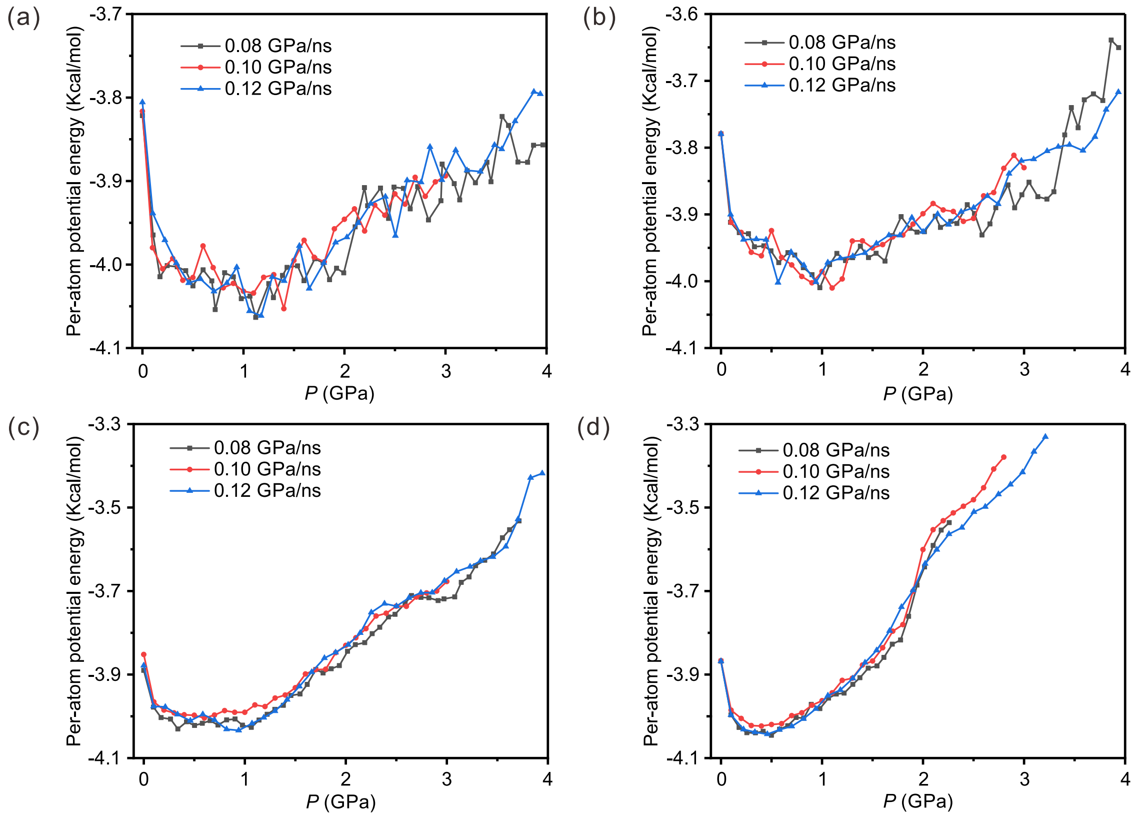


Figure S5: Variation of the potential energy of the confined water at different pressurization rates (0.08 GPa/ns, 0.10 GPa/ns, and 0.12 GPa/ns) during the pressurization process (the width of the capillary $h$ = 6.5 Å). (a) – (d) The size of graphene sheets is 26.6 Å × 21.9 Å, 42.5 Å × 35.0 Å, 68.0 Å × 56.0 Å, 108.8 Å × 89.6 Å, respectively.

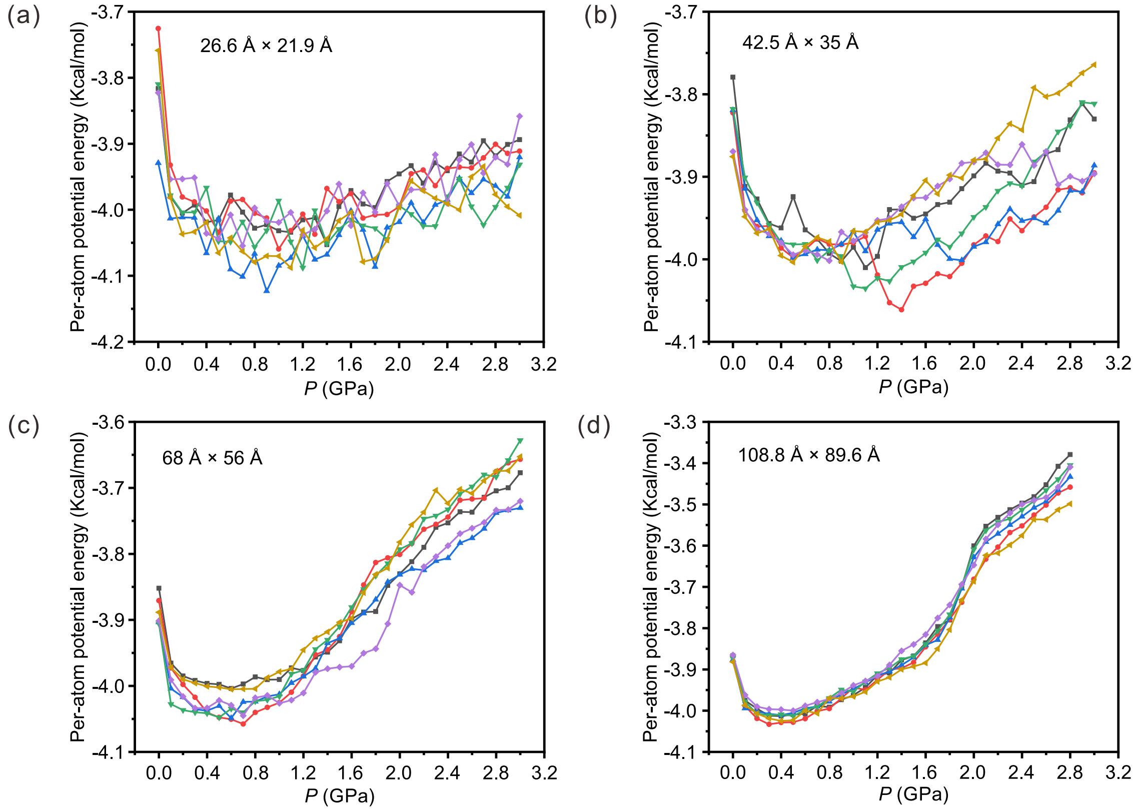


Figure S6: Variations of potential energy for different initial velocity distributions of the confined water during the pressurization process (the width of the capillary $h = 6.5$ Å). (a) – (d) The size of graphene sheets is 26.6 Å $\times$ 21.9 Å, 42.5 Å $\times$ 35.0 Å, 68.0 Å $\times$ 56.0 Å, 108.8 Å $\times$ 89.6 Å, respectively.

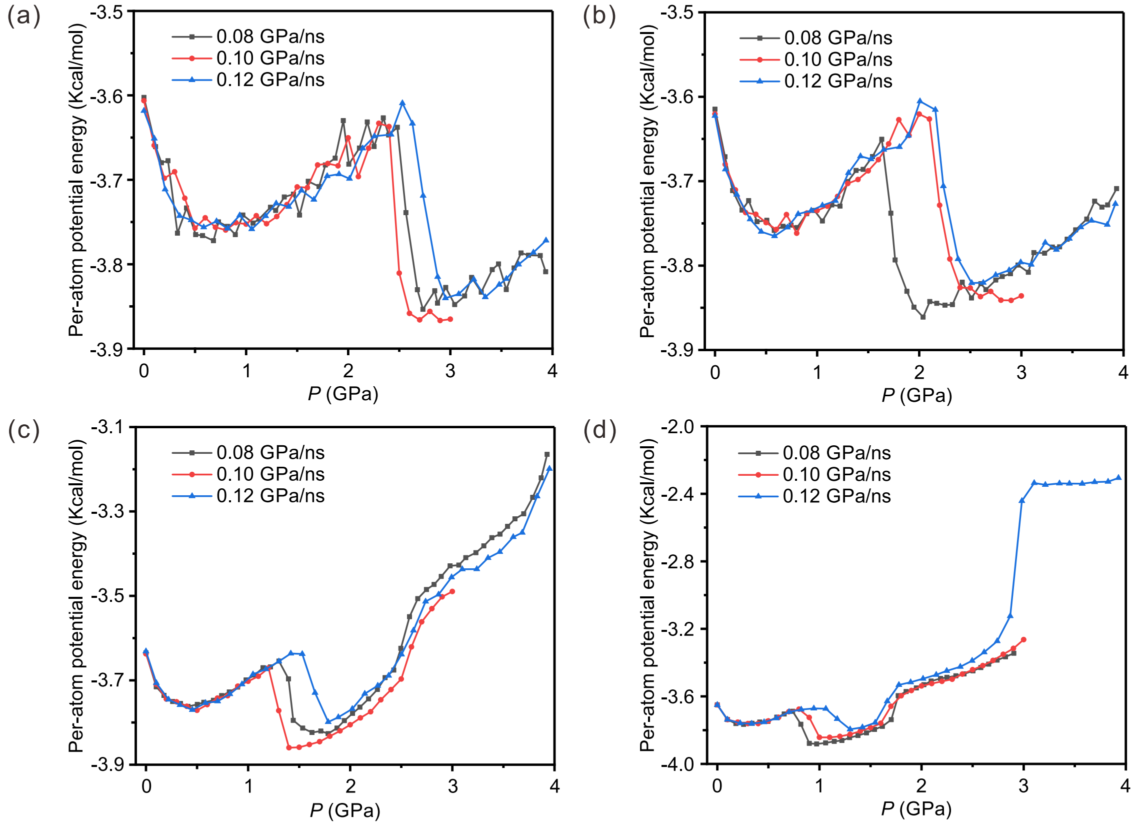


Figure S7: Variation of the potential energy of the confined water at different pressurization rates (0.08 GPa/ns, 0.10 GPa/ns, and 0.12 GPa/ns) during the pressurization process (the width of the capillary $h$ = 11.5 Å). (a) – (d) The size of graphene sheets is 26.6 Å × 21.9 Å, 42.5 Å × 35.0 Å, 68.0 Å × 56.0 Å, 108.8 Å × 89.6 Å, respectively.

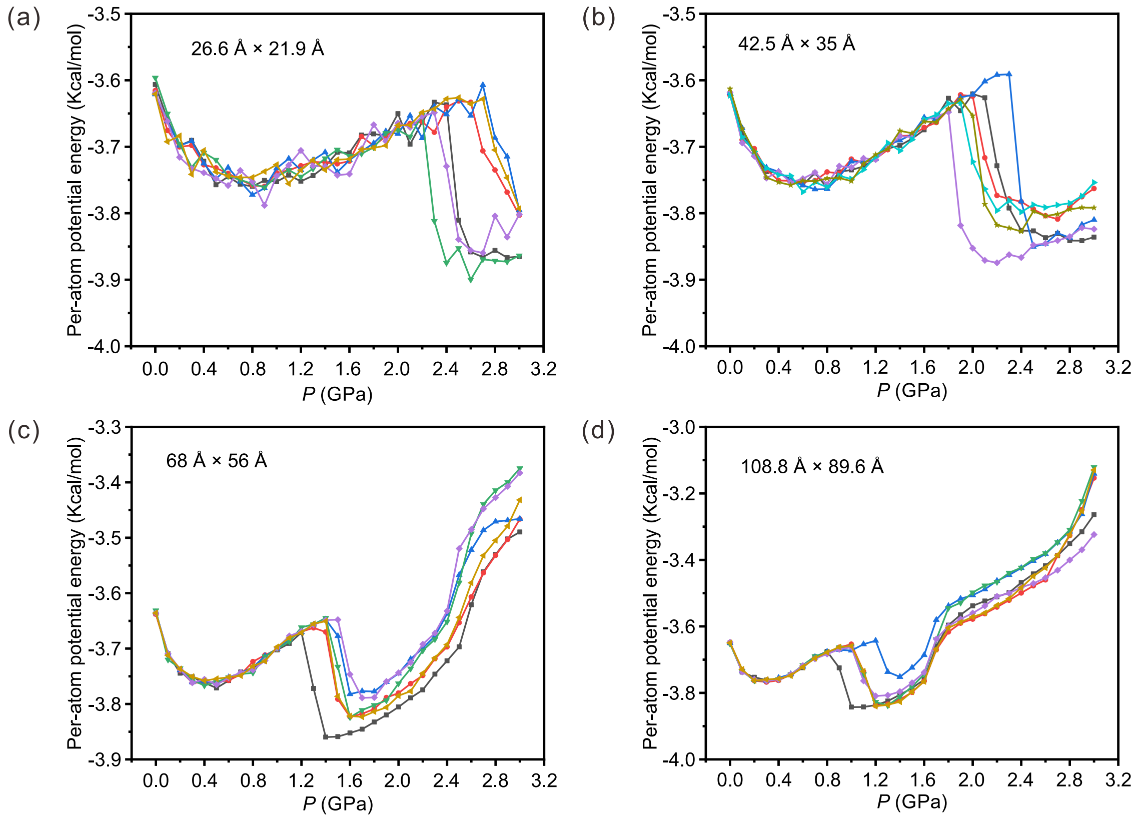


Figure S8: Variations of potential energy for different initial velocity distributions of the confined water during the pressurization process (the width of the capillary $h = 11.5$ Å). (a) – (d) The size of graphene sheets is 26.6 Å $\times$ 21.9 Å, 42.5 Å $\times$ 35.0 Å, 68.0 Å $\times$ 56.0 Å, 108.8 Å $\times$ 89.6 Å, respectively.
